# Supplementary material for: Distribution LMP-based Transactive Day-ahead Market with Variable Renewable Generation
Source: arXiv:1904.08998 source file (2019-04-18)
Supplement: Supplementary file 1 [file SUPPLEMENTAL.pdf]

# SUPPLEMENTAL SIMULATIONS

This document includes some additional simulation results as supplement to those reported in the manuscript.

Figure 1 shows simulation results for the base case reported as Scenario I in the manuscript.

Figure 2 represents simulation results for the case with $K = 4$ and $\alpha = 0.75$, reported as Scenario IV in the manuscript.

Each figure has been given a title to show what it depicts. The stair and horizontal black lines in "Power flow" and "Node pu voltage" figures show line MVA and normal voltage operation limits. All figures show quantities for 24 different timeslots. Load curtailments were only allowed if enough supply was not available to meet the total demand of the fixed segments (i.e., the first load segments). Hence, no curtailment has been observed in Scenario I (all load's fixed first segments were served). In Scenario IV, due to high VRE penetration, some VRE generation have been curtailed as voltage violations do not allow further penetration. During mid-hours some real power has been sold to the wholesale.

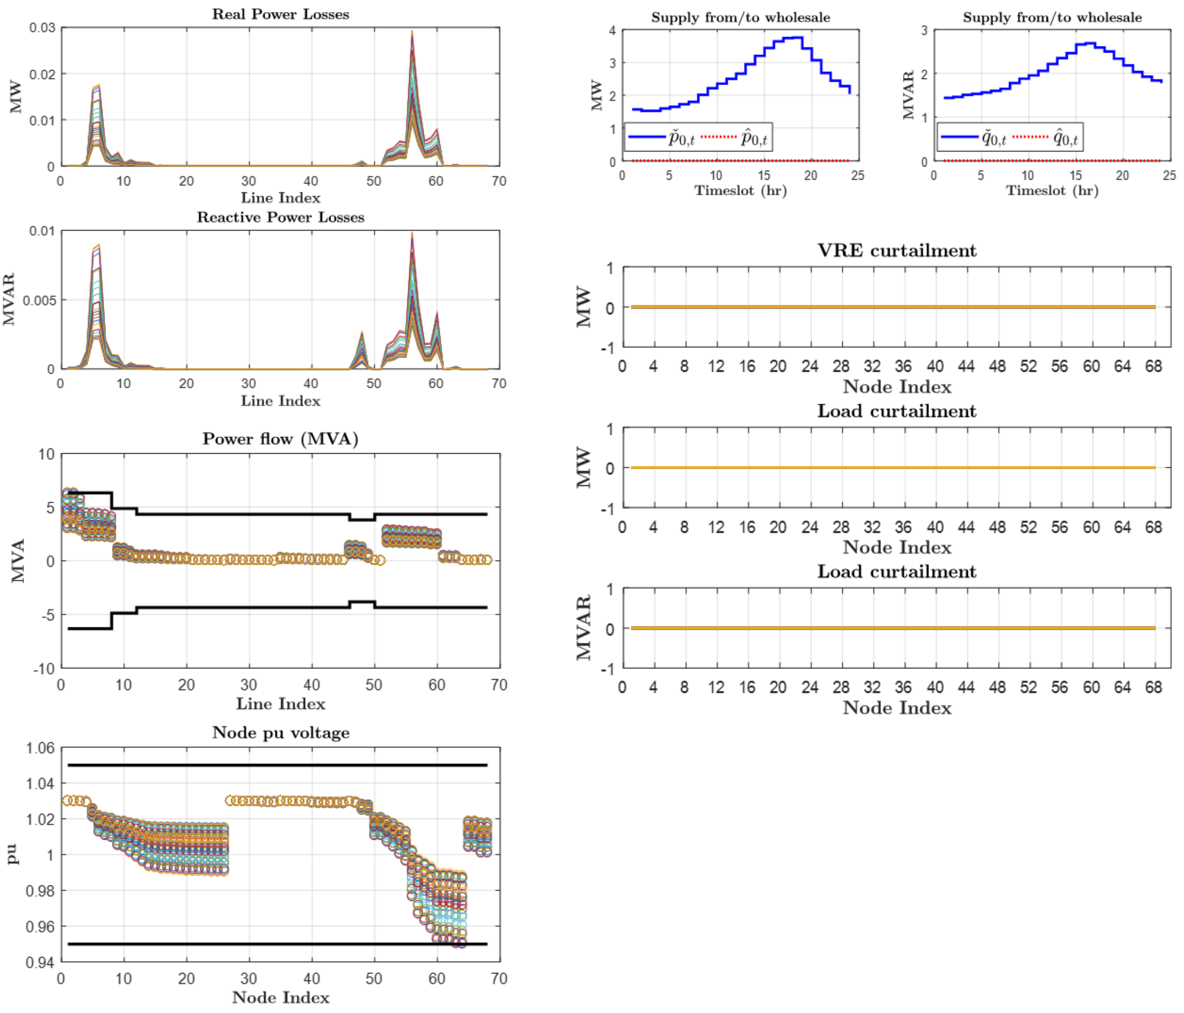


Figure 1: Simulation results under Scenario I.

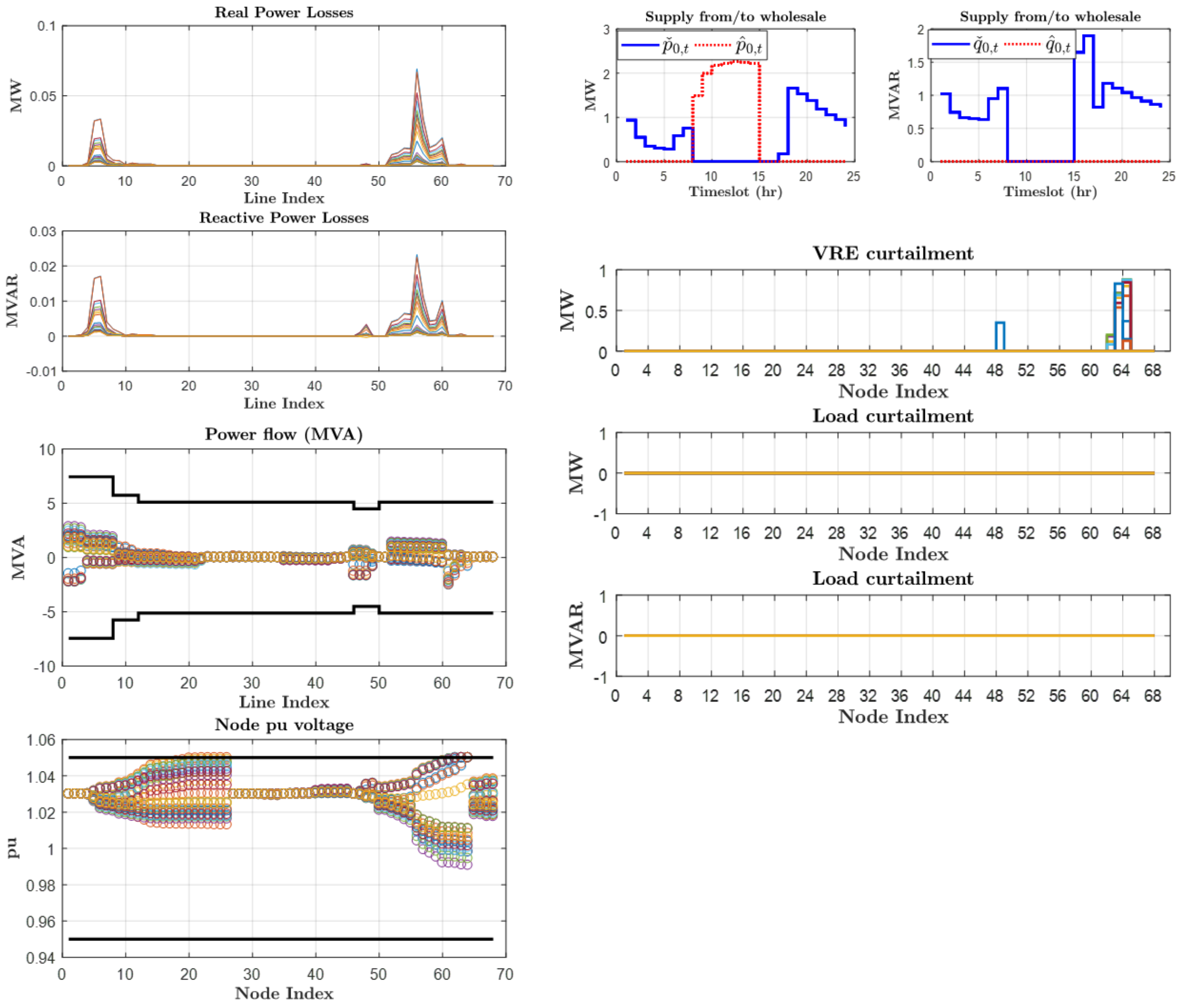


Figure 2: Simulation results under Scenario IV.
